# Supplementary material for: Bias Behind the Wheel: Fairness Testing of Autonomous Driving Systems
Source: arXiv:2308.02935 source file (2024-10-17)
Supplement: Supplementary file 1 [file appendix_figures.tex]

\begin{figure}[h]
\centering
\includegraphics[width=1\linewidth]{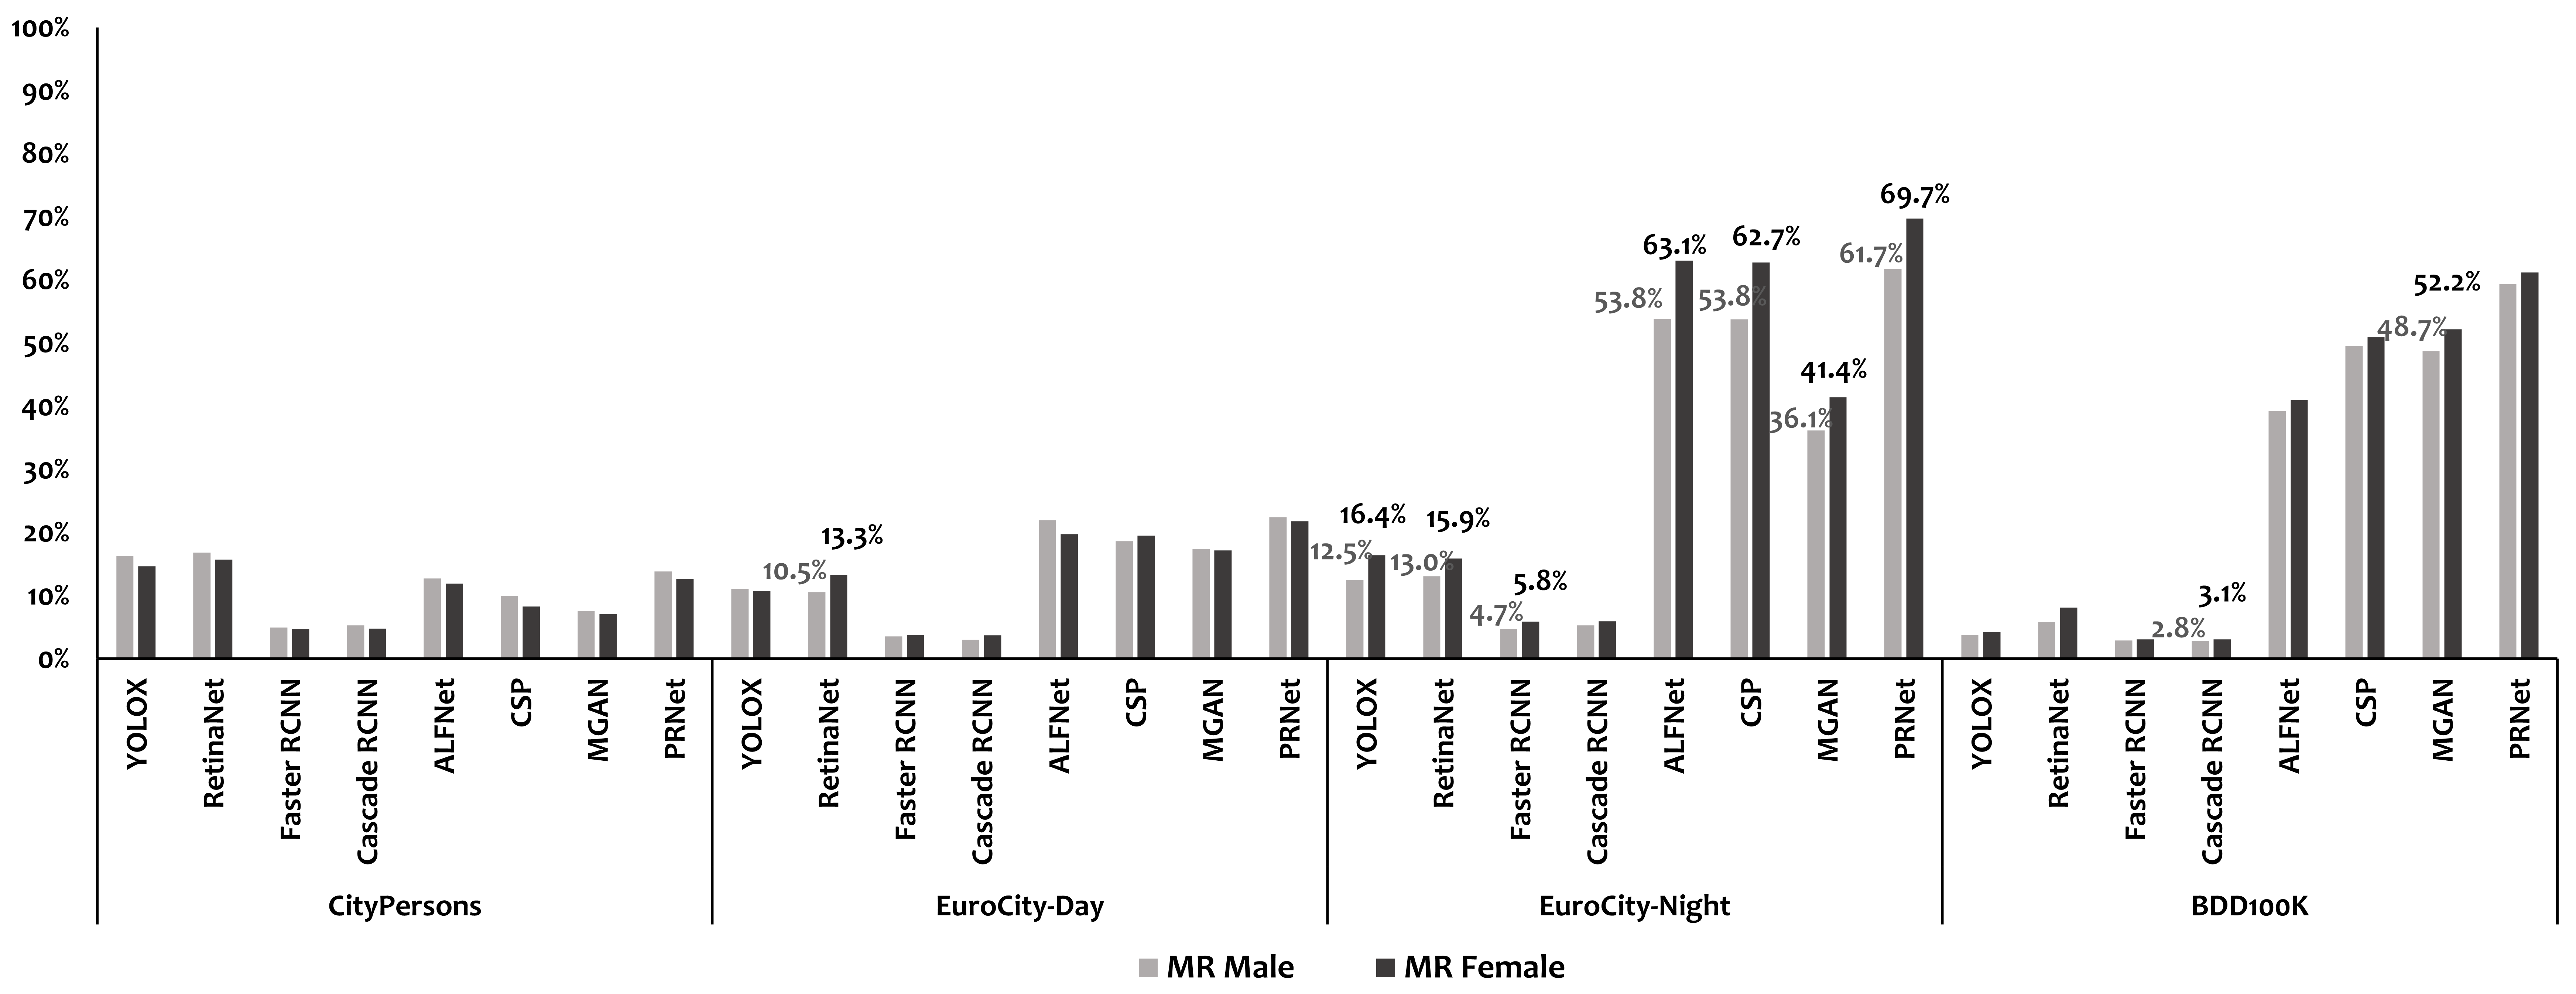}
\caption{\textit{RQ1: }Miss rates for female and male pedestrians in each dataset. Statistically significant gender unfairness (i.e., miss rate difference) is indicated by labeled miss rate values.}
\label{fig4:MR_gender_4datasets}
\end{figure}

\begin{figure}[h]
\centering
\includegraphics[width=1\linewidth]{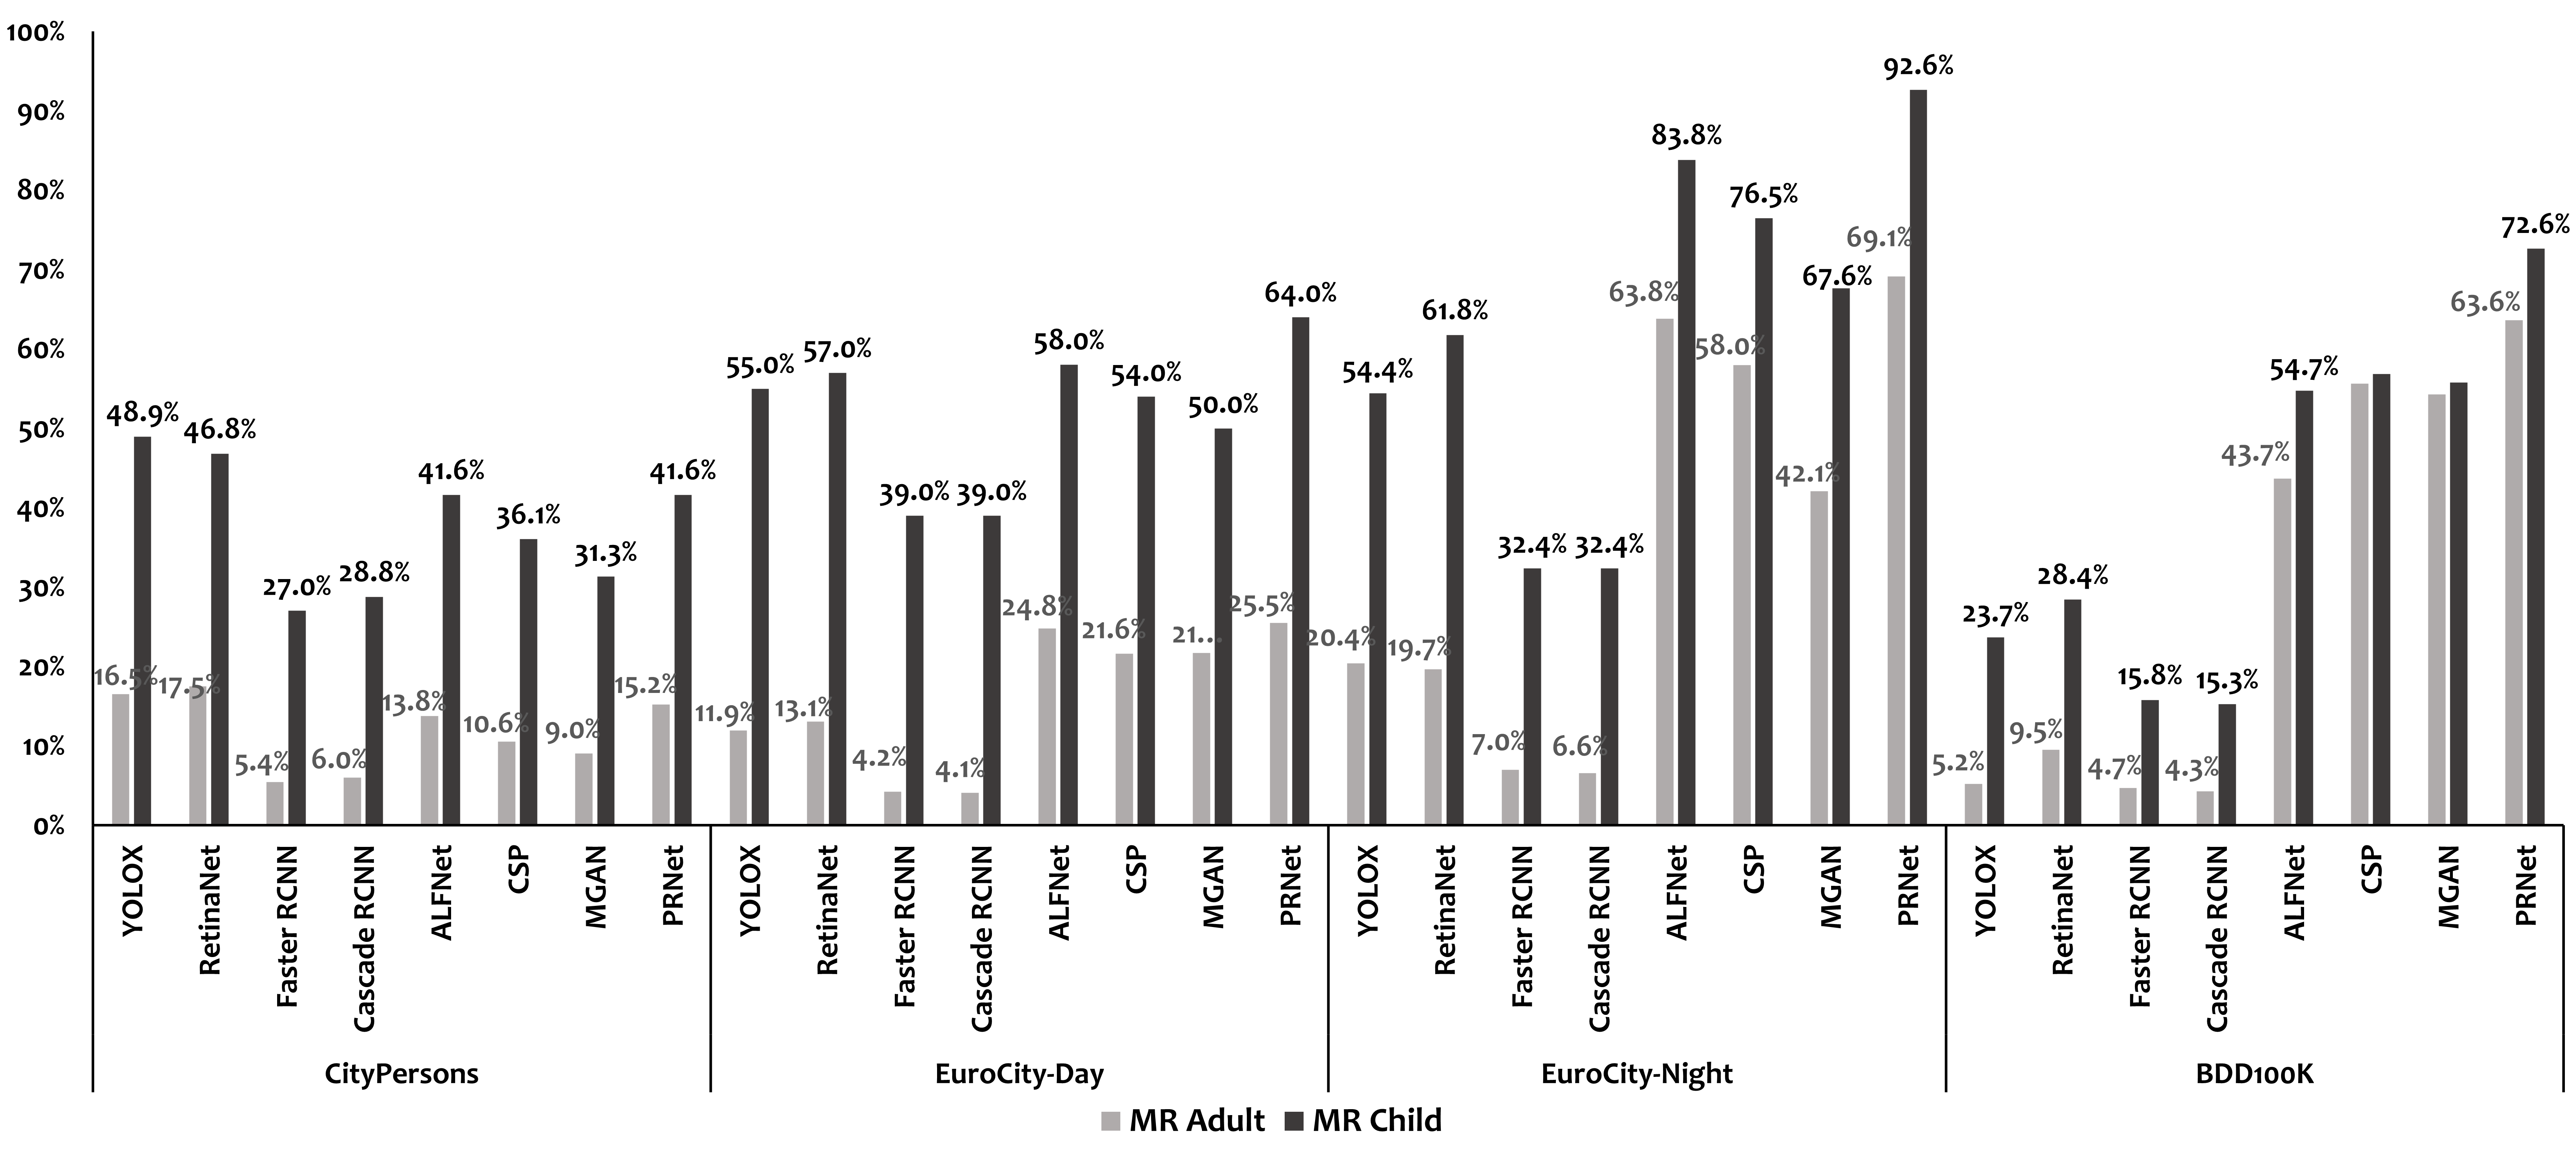}
\caption{\textit{RQ1: }Miss rates for children and adults in each dataset. Statistically significant age unfairness (i.e., miss rate difference) is indicated by labeled miss rate values.}
\label{fig5:MR_age_4datasets}
\end{figure}
